# Supplementary material for: Cosmic-ray propagation with DRAGON2: II. Nuclear interactions with the interstellar gas
Source: arXiv:1711.09616 ancillary file (2018-07-10)
Supplement: Supplementary file 1 [file ghost-nuclei.pdf]

## B Intermediate lived nuclei included in cross-section calculations in DRAGON2

| Stable or long<br>lived nucleus | Intermediate lived nuclei (branching ratio in %)                                                      |                                                                               |                |
|---------------------------------|-------------------------------------------------------------------------------------------------------|-------------------------------------------------------------------------------|----------------|
|                                 | 1st generation                                                                                        | 2nd generation                                                                | 3rd generation |
| $^2\text{H}$                    | $^{11}\text{Li}$ (0.013)<br>$^6\text{He}$ (0.01)                                                      |                                                                               |                |
| $^3\text{H}$                    | $^{11}\text{Li}$ (0.014)<br>$^8\text{He}$ (0.9)                                                       |                                                                               |                |
| $^4\text{He}$                   | $^8\text{B}$ (200.0)<br>$^{11}\text{Li}$ (1.0)<br>$^6\text{He}$ (0.01)                                |                                                                               |                |
| $^6\text{Li}$                   | $^6\text{He}$ (99.9)                                                                                  |                                                                               |                |
| $^7\text{Li}$                   | $^{11}\text{Be}$ (2.9)<br>$^8\text{He}$ (16.0)                                                        | $^{11}\text{Li}$ (8.07)                                                       |                |
| $^9\text{Be}$                   | $^9\text{Li}$ (49.2)<br>$^{11}\text{Li}$ (4.1)                                                        | $^{11}\text{Li}$ (0.013)                                                      |                |
| $^{10}\text{Be}$                | $^{11}\text{Li}$ (84.9)                                                                               |                                                                               |                |
| $^{10}\text{B}$                 | $^{10}\text{C}$ (100.0)                                                                               |                                                                               |                |
| $^{11}\text{B}$                 | $^{11}\text{C}$ (100.0)<br>$^{11}\text{Be}$ (97.1)<br>$^{12}\text{Be}$ (0.52)                         | $^{11}\text{Li}$ (8.07)                                                       |                |
| $^{12}\text{C}$                 | $^{13}\text{O}$ (10.9)<br>$^{12}\text{N}$ (96.5)<br>$^{12}\text{B}$ (98.4)<br>$^{13}\text{B}$ (0.279) | $^{12}\text{Be}$ (99.48)<br>$^{14}\text{Be}$ (5.0)<br>$^{14}\text{Be}$ (81.0) |                |

| Stable or long lived nucleus | Intermediate lived nuclei (branching ratio in %) |                         |                         |
|------------------------------|--------------------------------------------------|-------------------------|-------------------------|
|                              | 1st generation                                   | 2nd generation          | 3rd generation          |
| $^{13}\text{C}$              | $^{13}\text{N}$ (100.0)                          | $^{17}\text{Ne}$ (2.7)  |                         |
|                              |                                                  | $^{13}\text{O}$ (89.1)  |                         |
|                              | $^{17}\text{N}$ (0.01)                           | $^{17}\text{C}$ (71.59) | $^{17}\text{B}$ (22.1)  |
|                              |                                                  | $^{18}\text{C}$ (31.5)  |                         |
|                              |                                                  | $^{19}\text{C}$ (7.0)   | $^{19}\text{B}$ (100.0) |
|                              | $^{13}\text{B}$ (99.72)                          |                         |                         |
|                              | $^{14}\text{B}$ (6.04)                           | $^{14}\text{Be}$ (81.0) |                         |
|                              |                                                  | $^{14}\text{Be}$ (14.0) |                         |
|                              | $^{15}\text{B}$ (0.4)                            |                         |                         |
|                              | $^{17}\text{B}$ (0.4)                            |                         |                         |
| $^{14}\text{C}$              | $^{18}\text{N}$ (12.2)                           | $^{18}\text{C}$ (68.5)  |                         |
|                              |                                                  | $^{19}\text{C}$ (47.0)  | $^{19}\text{B}$ (100.0) |
|                              | $^{14}\text{B}$ (93.36)                          |                         |                         |
|                              | $^{15}\text{B}$ (93.6)                           | $^{14}\text{Be}$ (14.0) |                         |
|                              |                                                  | $^{17}\text{B}$ (3.5)   |                         |
| $^{14}\text{N}$              | $^{14}\text{O}$ (100.0)                          |                         |                         |
| $^{15}\text{N}$              | $^{15}\text{O}$ (100.0)                          | $^{15}\text{B}$ (6.0)   |                         |
|                              |                                                  | $^{17}\text{B}$ (11.0)  |                         |
|                              | $^{15}\text{C}$ (100.0)                          |                         |                         |
|                              |                                                  | $^{16}\text{C}$ (97.9)  | $^{17}\text{B}$ (63.0)  |
| $^{16}\text{O}$              | $^{20}\text{Na}$ (25.0)                          | $^{20}\text{Mg}$ (97.0) |                         |
|                              |                                                  |                         |                         |
|                              | $^{17}\text{Ne}$ (96.0)                          | $^{16}\text{C}$ (2.1)   | $^{17}\text{B}$ (63.0)  |
|                              |                                                  | $^{17}\text{C}$ (28.41) | $^{17}\text{B}$ (22.1)  |
|                              | $^{16}\text{N}$ (100.0)                          |                         |                         |
|                              |                                                  | $^{17}\text{C}$ (71.59) | $^{17}\text{B}$ (22.1)  |
|                              | $^{17}\text{N}$ (95.0)                           | $^{18}\text{C}$ (31.5)  |                         |
|                              |                                                  | $^{19}\text{C}$ (7.0)   | $^{19}\text{B}$ (100.0) |

| Stable or long lived nucleus | Intermediate lived nuclei (branching ratio in %) |                         |                          |
|------------------------------|--------------------------------------------------|-------------------------|--------------------------|
|                              | 1st generation                                   | 2nd generation          | 3rd generation           |
| $^{17}\text{O}$              | $^{17}\text{F}$ (100.0)                          | $^{21}\text{Mg}$ (0.5)  | $^{22}\text{Si}$ (32.0)  |
|                              |                                                  | $^{17}\text{Ne}$ (1.3)  |                          |
|                              |                                                  | $^{17}\text{N}$ (4.99)  | $^{17}\text{C}$ (71.59)  |
|                              | $^{18}\text{C}$ (31.5)                           |                         | $^{19}\text{B}$ (100.0)  |
|                              | $^{19}\text{C}$ (7.0)                            |                         |                          |
|                              | $^{18}\text{N}$ (10.9)                           | $^{18}\text{C}$ (68.5)  | $^{19}\text{B}$ (100.0)  |
| $^{19}\text{C}$ (47.0)       |                                                  |                         |                          |
| $^{18}\text{O}$              | $^{18}\text{N}$ (76.9)                           | $^{18}\text{C}$ (68.5)  | $^{19}\text{B}$ (100.0)  |
|                              |                                                  | $^{19}\text{C}$ (47.0)  |                          |
|                              | $^{19}\text{N}$ (54.6)                           | $^{19}\text{C}$ (46.0)  | $^{19}\text{B}$ (100.0)  |
|                              |                                                  | $^{20}\text{C}$ (72.0)  |                          |
|                              |                                                  | $^{18}\text{F}$         | $^{18}\text{Ne}$ (100.0) |
| $^{19}\text{F}$              | $^{19}\text{Ne}$ (100.0)                         | $^{20}\text{Mg}$ (3.0)  | $^{19}\text{C}$ (46.0)   |
|                              |                                                  | $^{19}\text{O}$ (100.0) |                          |
|                              | $^{19}\text{N}$ (45.4)                           | $^{20}\text{N}$ (56.99) | $^{20}\text{C}$ (28.0)   |
|                              |                                                  | $^{20}\text{N}$ (56.99) |                          |
|                              |                                                  | $^{20}\text{N}$ (56.99) |                          |
| $^{20}\text{Ne}$             | $^{22}\text{Al}$ (2.5)                           | $^{22}\text{Si}$ (68.0) |                          |
|                              | $^{24}\text{Al}$ (0.0349)                        | $^{24}\text{Si}$ (92.0) |                          |
|                              | $^{21}\text{Mg}$ (32.6)                          | $^{22}\text{Si}$ (32.0) |                          |
|                              | $^{20}\text{Na}$ (75.0)                          | $^{20}\text{Mg}$ (97.0) |                          |
|                              | $^{20}\text{F}$ (100.0)                          | $^{20}\text{O}$ (100.0) | $^{20}\text{N}$ (43.0)   |
|                              |                                                  | $^{20}\text{O}$ (100.0) | $^{21}\text{N}$ (80.0)   |
|                              |                                                  | $^{20}\text{O}$ (100.0) |                          |

| Stable or long lived nucleus | Intermediate lived nuclei (branching ratio in %) |                          |                          |
|------------------------------|--------------------------------------------------|--------------------------|--------------------------|
|                              | 1st generation                                   | 2nd generation           | 3rd generation           |
| $^{21}\text{Ne}$             | $^{21}\text{Na}$ (100.0)                         | $^{22}\text{Al}$ (0.8)   | $^{22}\text{Si}$ (68.0)  |
|                              |                                                  | $^{21}\text{Mg}$ (66.9)  | $^{22}\text{Si}$ (32.0)  |
|                              | $^{21}\text{F}$ (100.0)                          | $^{21}\text{O}$ (100.0)  | $^{21}\text{N}$ (20.0)   |
|                              |                                                  | $^{22}\text{O}$ (22.0)   | $^{22}\text{N}$ (35.0)   |
|                              |                                                  | $^{22}\text{N}$ (65.0)   |                          |
|                              | $^{22}\text{F}$ (11.0)                           | $^{22}\text{O}$ (78.0)   | $^{22}\text{N}$ (65.0)   |
|                              |                                                  | $^{23}\text{O}$ (58.0)   | $^{23}\text{N}$ (100.0)  |
|                              |                                                  |                          |                          |
|                              |                                                  |                          |                          |
|                              | $^{22}\text{Ne}$                                 | $^{22}\text{F}$ (89.0)   | $^{22}\text{O}$ (78.0)   |
| $^{23}\text{O}$ (58.0)       |                                                  |                          | $^{23}\text{N}$ (100.0)  |
| $^{23}\text{F}$ (14.0)       |                                                  | $^{23}\text{O}$ (42.0)   | $^{23}\text{N}$ (100.0)  |
|                              |                                                  | $^{24}\text{O}$ (57.99)  |                          |
|                              |                                                  |                          |                          |
|                              |                                                  |                          |                          |
| $^{22}\text{Na}$             | $^{23}\text{Al}$ (8.0)                           | $^{23}\text{Si}$ (100.0) |                          |
|                              | $^{22}\text{Mg}$ (100.0)                         | $^{22}\text{Al}$ (96.7)  | $^{22}\text{Si}$ (68.0)  |
|                              |                                                  |                          |                          |
|                              |                                                  |                          |                          |
| $^{23}\text{Na}$             | $^{24}\text{Al}$ (0.0159)                        | $^{24}\text{Si}$ (92.0)  |                          |
|                              |                                                  | $^{23}\text{Si}$ (8.0)   |                          |
|                              | $^{23}\text{Mg}$ (100.0)                         | $^{23}\text{Al}$ (92.0)  | $^{23}\text{Si}$ (100.0) |
|                              |                                                  |                          |                          |
|                              | $^{23}\text{Ne}$ (100.0)                         | $^{23}\text{F}$ (86.0)   | $^{23}\text{O}$ (42.0)   |
|                              |                                                  |                          | $^{24}\text{O}$ (57.99)  |
|                              |                                                  | $^{24}\text{F}$ (5.9)    | $^{24}\text{O}$ (42.01)  |
|                              |                                                  |                          |                          |
| $^{24}\text{Na}$             | $^{24}\text{Ne}$ (100.0)                         | $^{24}\text{F}$ (94.1)   | $^{24}\text{O}$ (42.01)  |
|                              |                                                  | $^{25}\text{F}$ (24.0)   |                          |
|                              |                                                  |                          |                          |

| Stable or long lived nucleus | Intermediate lived nuclei (branching ratio in %)                                 |                                                                                                                                           |                                                                                                                |
|------------------------------|----------------------------------------------------------------------------------|-------------------------------------------------------------------------------------------------------------------------------------------|----------------------------------------------------------------------------------------------------------------|
|                              | 1st generation                                                                   | 2nd generation                                                                                                                            | 3rd generation                                                                                                 |
| $^{24}\text{Mg}$             | $^{26}\text{P}$ (1.0)<br>$^{25}\text{Si}$ (36.8)<br>$^{24}\text{Al}$ (99.95)     | $^{24}\text{Si}$ (92.0)                                                                                                                   |                                                                                                                |
| $^{25}\text{Mg}$             | $^{25}\text{Al}$ (100.0)<br><br>$^{25}\text{Na}$ (100.0)                         | $^{27}\text{S}$ (2.0)<br>$^{26}\text{P}$ (0.9)<br>$^{25}\text{Si}$ (63.19)<br><br>$^{25}\text{Ne}$ (100.0)<br><br>$^{26}\text{Ne}$ (0.13) | $^{25}\text{F}$ (76.0)<br>$^{26}\text{F}$ (32.0)<br><br>$^{30}\text{Na}$ (0.5)<br>$^{26}\text{F}$ (68.0)       |
| $^{26}\text{Mg}$             | $^{26}\text{Na}$ (100.0)<br><br>$^{27}\text{Na}$ (0.13)                          | $^{26}\text{Ne}$ (99.87)<br><br>$^{27}\text{Ne}$ (2.0)<br><br>$^{27}\text{Ne}$ (98.0)<br><br>$^{28}\text{Ne}$ (22.0)                      | $^{30}\text{Na}$ (0.5)<br>$^{26}\text{F}$ (68.0)<br><br>$^{27}\text{F}$ (100.0)<br><br>$^{27}\text{F}$ (100.0) |
| $^{28}\text{Mg}$             | $^{28}\text{Na}$ (99.421)<br>$^{29}\text{Na}$ (25.91)<br>$^{30}\text{Na}$ (1.17) | $^{28}\text{Ne}$ (78.0)<br>$^{29}\text{Ne}$ (100.0)<br><br>$^{30}\text{Ne}$ (100.0)                                                       | $^{29}\text{F}$ (100.0)                                                                                        |
| $^{26}\text{Al}$             | $^{27}\text{P}$ (0.07)<br>$^{26}\text{Si}$ (100.0)                               | $^{27}\text{S}$ (98.0)<br><br>$^{26}\text{P}$ (98.1)                                                                                      |                                                                                                                |

| Stable or long lived nucleus | Intermediate lived nuclei (branching ratio in %) |                          |                          |
|------------------------------|--------------------------------------------------|--------------------------|--------------------------|
|                              | 1st generation                                   | 2nd generation           | 3rd generation           |
| $^{27}\text{Al}$             | $^{28}\text{P}$ (0.01)                           |                          |                          |
|                              | $^{27}\text{Si}$ (100.0)                         | $^{28}\text{S}$ (79.3)   |                          |
|                              |                                                  | $^{28}\text{S}$ (20.7)   |                          |
|                              |                                                  | $^{27}\text{P}$ (99.93)  | $^{27}\text{S}$ (98.0)   |
|                              | $^{27}\text{Mg}$ (100.0)                         | $^{27}\text{Na}$ (99.87) | $^{27}\text{Ne}$ (98.0)  |
|                              |                                                  | $^{28}\text{Na}$ (0.579) | $^{28}\text{Ne}$ (22.0)  |
|                              |                                                  | $^{28}\text{Ne}$ (78.0)  |                          |
| $^{28}\text{Si}$             | $^{31}\text{Ar}$ (2.1)                           |                          |                          |
|                              | $^{32}\text{Cl}$ (0.054)                         |                          |                          |
|                              | $^{29}\text{S}$ (46.4)                           | $^{32}\text{Ar}$ (56.99) |                          |
|                              | $^{28}\text{P}$ (99.99)                          |                          |                          |
|                              | $^{28}\text{Al}$ (100.0)                         | $^{28}\text{S}$ (79.3)   |                          |
| $^{29}\text{Si}$             | $^{29}\text{P}$ (100.0)                          | $^{31}\text{Ar}$ (2.48)  |                          |
|                              |                                                  | $^{29}\text{S}$ (53.6)   |                          |
|                              | $^{29}\text{Al}$ (100.0)                         | $^{29}\text{Mg}$ (100.0) | $^{29}\text{Na}$ (74.09) |
|                              |                                                  |                          | $^{30}\text{Na}$ (30.0)  |
|                              |                                                  | $^{30}\text{Mg}$ (0.06)  | $^{30}\text{Na}$ (68.33) |
|                              |                                                  |                          | $^{31}\text{Na}$ (37.95) |
| $^{30}\text{Si}$             | $^{30}\text{P}$ (100.0)                          | $^{31}\text{Cl}$ (0.7)   | $^{31}\text{Ar}$ (40.4)  |
|                              |                                                  | $^{30}\text{S}$ (100.0)  | $^{31}\text{Ar}$ (55.0)  |
|                              | $^{30}\text{Al}$ (100.0)                         | $^{30}\text{Mg}$ (99.94) | $^{30}\text{Na}$ (68.33) |
|                              |                                                  |                          | $^{31}\text{Na}$ (37.95) |
|                              |                                                  | $^{31}\text{Mg}$ (1.7)   | $^{31}\text{Na}$ (62.05) |
|                              |                                                  |                          | $^{33}\text{Na}$ (12.0)  |
|                              | $^{31}\text{Al}$ (1.6)                           | $^{31}\text{Mg}$ (98.3)  | $^{31}\text{Na}$ (62.05) |
|                              |                                                  |                          | $^{33}\text{Na}$ (12.0)  |
|                              |                                                  | $^{32}\text{Mg}$ (2.4)   | $^{33}\text{Na}$ (52.0)  |
|                              |                                                  |                          | $^{34}\text{Na}$ (50.0)  |

| Stable or long lived nucleus | Intermediate lived nuclei (branching ratio in %)     |                          |                                                     |
|------------------------------|------------------------------------------------------|--------------------------|-----------------------------------------------------|
|                              | 1st generation                                       | 2nd generation           | 3rd generation                                      |
| $^{31}\text{Si}$             | $^{31}\text{Al}$ (98.4)                              | $^{31}\text{Mg}$ (98.3)  | $^{31}\text{Na}$ (62.05)<br>$^{33}\text{Na}$ (12.0) |
|                              |                                                      | $^{32}\text{Mg}$ (2.4)   | $^{33}\text{Na}$ (52.0)<br>$^{34}\text{Na}$ (50.0)  |
|                              | $^{32}\text{Al}$ (0.7)                               | $^{32}\text{Mg}$ (97.6)  | $^{33}\text{Na}$ (52.0)<br>$^{34}\text{Na}$ (50.0)  |
|                              |                                                      | $^{33}\text{Mg}$ (17.0)  | $^{33}\text{Na}$ (36.0)<br>$^{34}\text{Na}$ (15.0)  |
|                              |                                                      |                          |                                                     |
|                              |                                                      |                          |                                                     |
| $^{32}\text{Si}$             | $^{32}\text{Al}$ (99.3)                              | $^{32}\text{Mg}$ (97.6)  | $^{33}\text{Na}$ (52.0)<br>$^{34}\text{Na}$ (50.0)  |
|                              |                                                      | $^{33}\text{Mg}$ (17.0)  | $^{33}\text{Na}$ (36.0)<br>$^{34}\text{Na}$ (15.0)  |
|                              | $^{33}\text{Al}$ (8.5)                               | $^{33}\text{Mg}$ (83.0)  | $^{33}\text{Na}$ (36.0)<br>$^{34}\text{Na}$ (15.0)  |
|                              |                                                      |                          |                                                     |
|                              |                                                      |                          |                                                     |
|                              |                                                      |                          |                                                     |
| $^{31}\text{P}$              | $^{32}\text{Cl}$ (0.026)                             | $^{32}\text{Ar}$ (56.99) | $^{31}\text{Ar}$ (40.4)                             |
|                              | $^{31}\text{S}$ (100.0)                              |                          |                                                     |
|                              |                                                      |                          |                                                     |
|                              |                                                      |                          |                                                     |
| $^{33}\text{P}$              | $^{33}\text{Si}$ (100.0)                             | $^{33}\text{Al}$ (91.5)  | $^{33}\text{Mg}$ (83.0)                             |
|                              |                                                      | $^{34}\text{Al}$ (12.5)  | $^{34}\text{Mg}$ (100.0)<br>$^{35}\text{Mg}$ (52.0) |
|                              |                                                      |                          |                                                     |
| $^{32}\text{S}$              | $^{36}\text{K}$ (0.012)                              | $^{36}\text{Ca}$ (43.2)  |                                                     |
|                              | $^{33}\text{Ar}$ (38.65)<br>$^{32}\text{Cl}$ (99.92) |                          |                                                     |
|                              |                                                      |                          |                                                     |

| Stable or long lived nucleus | Intermediate lived nuclei (branching ratio in %) |                          |                          |
|------------------------------|--------------------------------------------------|--------------------------|--------------------------|
|                              | 1st generation                                   | 2nd generation           | 3rd generation           |
| $^{33}\text{S}$              | $^{33}\text{Cl}$ (100.0)                         | $^{33}\text{Ar}$ (61.35) |                          |
| $^{34}\text{S}$              | $^{34}\text{Cl}$ (100.0)                         | $^{35}\text{K}$ (0.37)   | $^{35}\text{Ca}$ (100.0) |
|                              | $^{34}\text{P}$ (100.0)                          | $^{34}\text{Ar}$ (100.0) |                          |
|                              |                                                  | $^{34}\text{Si}$ (100.0) | $^{34}\text{Al}$ (87.5)  |
|                              |                                                  | $^{35}\text{Si}$ (5.26)  | $^{35}\text{Al}$ (26.0)  |
|                              |                                                  |                          | $^{35}\text{Al}$ (74.0)  |
|                              |                                                  |                          | $^{36}\text{Al}$ (31.0)  |
| $^{35}\text{S}$              | $^{35}\text{P}$ (100.0)                          | $^{35}\text{Si}$ (94.74) | $^{35}\text{Al}$ (74.0)  |
|                              |                                                  |                          | $^{36}\text{Al}$ (31.0)  |
|                              |                                                  | $^{36}\text{Si}$ (12.0)  | $^{36}\text{Al}$ (69.0)  |
| $^{36}\text{S}$              | $^{36}\text{P}$ (100.0)                          | $^{36}\text{Si}$ (88.0)  | $^{36}\text{Al}$ (69.0)  |
|                              |                                                  | $^{37}\text{Si}$ (17.0)  | $^{37}\text{Al}$ (100.0) |
| $^{35}\text{Cl}$             | $^{36}\text{K}$ (0.048)                          | $^{36}\text{Ca}$ (43.2)  |                          |
|                              | $^{35}\text{Ar}$ (100.0)                         | $^{36}\text{Ca}$ (56.8)  |                          |
|                              |                                                  | $^{35}\text{K}$ (99.63)  | $^{35}\text{Ca}$ (100.0) |
| $^{37}\text{Cl}$             | $^{37}\text{S}$ (100.0)                          | $^{37}\text{P}$ (100.0)  | $^{37}\text{Si}$ (83.0)  |
|                              |                                                  | $^{38}\text{P}$ (12.0)   |                          |
| $^{36}\text{Ar}$             | $^{40}\text{Sc}$ (0.02)                          | $^{40}\text{Ti}$ (57.0)  |                          |
|                              | $^{37}\text{Ca}$ (74.5)                          |                          |                          |
|                              | $^{36}\text{K}$ (99.94)                          | $^{36}\text{Ca}$ (43.2)  |                          |
| $^{37}\text{Ar}$             | $^{37}\text{K}$ (100.0)                          | $^{37}\text{Ca}$ (25.5)  |                          |

| Stable or long lived nucleus | Intermediate lived nuclei (branching ratio in %) |                          |                         |
|------------------------------|--------------------------------------------------|--------------------------|-------------------------|
|                              | 1st generation                                   | 2nd generation           | 3rd generation          |
| $^{38}\text{Ar}$             | $^{38}\text{K}$ (100.0)                          | $^{38}\text{Ca}$ (100.0) | $^{39}\text{Ti}$ (85.0) |
|                              |                                                  |                          | $^{38}\text{P}$ (88.0)  |
|                              | $^{38}\text{Cl}$ (100.0)                         | $^{38}\text{S}$ (100.0)  | $^{39}\text{P}$ (26.0)  |
|                              |                                                  |                          |                         |
| $^{39}\text{Ar}$             | $^{39}\text{Cl}$ (100.0)                         | $^{39}\text{S}$ (100.0)  | $^{39}\text{P}$ (74.0)  |
|                              |                                                  |                          | $^{40}\text{P}$ (30.0)  |
|                              |                                                  |                          |                         |
| $^{40}\text{Ar}$             | $^{40}\text{Cl}$ (100.0)                         | $^{40}\text{S}$ (100.0)  | $^{40}\text{P}$ (70.0)  |
|                              |                                                  |                          | $^{41}\text{P}$ (30.0)  |
|                              |                                                  |                          |                         |
| $^{41}\text{Ar}$             | $^{41}\text{Cl}$ (100.0)                         | $^{41}\text{S}$ (100.0)  | $^{41}\text{P}$ (70.0)  |
|                              |                                                  |                          | $^{42}\text{P}$ (50.0)  |
|                              |                                                  | $^{42}\text{S}$ (4.0)    | $^{42}\text{P}$ (50.0)  |
|                              |                                                  |                          | $^{43}\text{P}$ (100.0) |
|                              |                                                  |                          |                         |
| $^{42}\text{Ar}$             | $^{42}\text{Cl}$ (100.0)                         | $^{42}\text{S}$ (96.0)   | $^{42}\text{P}$ (50.0)  |
|                              |                                                  |                          | $^{43}\text{P}$ (100.0) |
|                              |                                                  | $^{43}\text{S}$ (40.0)   |                         |
|                              |                                                  |                          |                         |
| $^{39}\text{K}$              | $^{40}\text{Sc}$ (0.48)                          | $^{40}\text{Ti}$ (57.0)  |                         |
|                              | $^{39}\text{Ca}$ (100.0)                         |                          | $^{40}\text{Ti}$ (43.0) |
|                              |                                                  |                          |                         |
| $^{43}\text{K}$              | $^{43}\text{Ar}$ (100.0)                         | $^{43}\text{Cl}$ (100.0) | $^{43}\text{S}$ (60.0)  |
|                              |                                                  |                          | $^{44}\text{S}$ (18.0)  |
|                              |                                                  | $^{44}\text{Cl}$ (8.0)   | $^{44}\text{S}$ (82.0)  |
|                              |                                                  |                          | $^{45}\text{S}$ (54.0)  |
|                              |                                                  |                          |                         |

| Stable or long lived nucleus | Intermediate lived nuclei (branching ratio in %)    |                                                      |                                                                              |
|------------------------------|-----------------------------------------------------|------------------------------------------------------|------------------------------------------------------------------------------|
|                              | 1st generation                                      | 2nd generation                                       | 3rd generation                                                               |
| $^{40}\text{Ca}$             | $^{41}\text{Ti}$ (100.0)<br>$^{40}\text{Sc}$ (99.5) | $^{40}\text{Ti}$ (57.0)                              |                                                                              |
| $^{41}\text{Ca}$             | $^{41}\text{Sc}$ (100.0)                            | $^{43}\text{Cr}$ (6.0)                               | $^{45}\text{Fe}$ (70.0)                                                      |
| $^{42}\text{Ca}$             | $^{42}\text{Sc}$ (100.0)                            | $^{42}\text{Ti}$ (100.0)                             | $^{43}\text{Cr}$ (23.0)                                                      |
| $^{44}\text{Ca}$             | $^{44}\text{K}$ (100.0)                             | $^{44}\text{Ar}$ (100.0)                             | $^{44}\text{Cl}$ (92.0)<br>$^{45}\text{Cl}$ (24.0)                           |
| $^{45}\text{Ca}$             | $^{45}\text{K}$ (100.0)                             | $^{45}\text{Ar}$ (100.0)                             | $^{45}\text{Cl}$ (76.0)<br>$^{46}\text{Cl}$ (60.0)                           |
| $^{46}\text{Ca}$             | $^{46}\text{K}$ (100.0)                             | $^{46}\text{Ar}$ (100.0)<br>$^{47}\text{Ar}$ (1.0)   | $^{46}\text{Cl}$ (40.0)<br>$^{47}\text{Cl}$ (3.0)<br>$^{47}\text{Cl}$ (97.0) |
| $^{47}\text{Ca}$             | $^{47}\text{K}$ (100.0)<br>$^{48}\text{K}$ (1.14)   | $^{47}\text{Ar}$ (99.0)<br>$^{48}\text{Ar}$ (100.0)  | $^{47}\text{Cl}$ (97.0)                                                      |
| $^{48}\text{Ca}$             | $^{48}\text{K}$ (98.86)<br>$^{49}\text{K}$ (86.0)   | $^{48}\text{Ar}$ (100.0)<br>$^{49}\text{Ar}$ (100.0) |                                                                              |
| $^{43}\text{Sc}$             | $^{43}\text{Ti}$ (100.0)                            | $^{44}\text{Cr}$ (7.0)                               |                                                                              |
| $^{44}\text{Ti}$             | $^{45}\text{Cr}$ (27.0)<br>$^{44}\text{V}$ (100.0)  | $^{44}\text{Cr}$ (93.0)                              |                                                                              |

| Stable or long lived nucleus | Intermediate lived nuclei (branching ratio in %)   |                                                     |                                                                              |
|------------------------------|----------------------------------------------------|-----------------------------------------------------|------------------------------------------------------------------------------|
|                              | 1st generation                                     | 2nd generation                                      | 3rd generation                                                               |
| $^{45}\text{Ti}$             | $^{45}\text{V}$ (100.0)                            | $^{46}\text{Mn}$ (22.0)<br>$^{45}\text{Cr}$ (73.0)  | $^{46}\text{Fe}$ (100.0)                                                     |
| $^{46}\text{Ti}$             | $^{46}\text{V}$ (100.0)                            | $^{47}\text{Mn}$ (3.4)<br>$^{46}\text{Cr}$ (100.0)  | $^{47}\text{Fe}$ (100.0)<br>$^{46}\text{Mn}$ (78.0)                          |
| $^{47}\text{Ti}$             | $^{47}\text{V}$ (100.0)                            | $^{48}\text{Mn}$ (0.03)<br>$^{47}\text{Cr}$ (100.0) | $^{48}\text{Fe}$ (96.4)<br>$^{48}\text{Fe}$ (3.6)<br>$^{47}\text{Mn}$ (96.6) |
| $^{49}\text{Ti}$             | $^{49}\text{Sc}$ (100.0)                           | $^{49}\text{Ca}$ (100.0)                            | $^{49}\text{K}$ (14.0)<br>$^{50}\text{K}$ (29.0)                             |
| $^{50}\text{Ti}$             | $^{50}\text{Sc}$ (100.0)                           | $^{50}\text{Ca}$ (100.0)                            | $^{50}\text{K}$ (71.0)<br>$^{51}\text{K}$ (47.0)<br>$^{52}\text{K}$ (21.0)   |
| $^{49}\text{V}$              | $^{49}\text{Cr}$ (100.0)                           | $^{49}\text{Mn}$ (100.0)                            | $^{49}\text{Fe}$ (48.0)                                                      |
| $^{51}\text{V}$              | $^{51}\text{Ti}$ (100.0)                           | $^{51}\text{Sc}$ (100.0)                            | $^{51}\text{Ca}$ (100.0)<br>$^{52}\text{Ca}$ (2.0)                           |
| $^{48}\text{Cr}$             | $^{49}\text{Fe}$ (52.0)<br>$^{48}\text{Mn}$ (99.7) | $^{48}\text{Fe}$ (96.4)                             |                                                                              |
| $^{50}\text{Cr}$             | $^{50}\text{Mn}$ (100.0)                           | $^{50}\text{Fe}$ (100.0)                            |                                                                              |

| Stable or long lived nucleus | Intermediate lived nuclei (branching ratio in %) |                          |                          |
|------------------------------|--------------------------------------------------|--------------------------|--------------------------|
|                              | 1st generation                                   | 2nd generation           | 3rd generation           |
| $^{51}\text{Cr}$             | $^{51}\text{Mn}$ (100.0)                         | $^{51}\text{Fe}$ (100.0) |                          |
| $^{52}\text{Cr}$             | $^{52}\text{V}$ (100.0)                          | $^{52}\text{Ti}$ (100.0) | $^{52}\text{Sc}$ (100.0) |
| $^{53}\text{Cr}$             | $^{53}\text{V}$ (100.0)                          | $^{53}\text{Ti}$ (100.0) | $^{53}\text{Sc}$ (100.0) |
| $^{54}\text{Cr}$             | $^{54}\text{V}$ (100.0)                          | $^{54}\text{Ti}$ (100.0) | $^{54}\text{Sc}$ (100.0) |
| $^{53}\text{Mn}$             | $^{53}\text{Fe}$ (100.0)                         |                          |                          |
| $^{55}\text{Mn}$             | $^{55}\text{Cr}$ (100.0)                         | $^{55}\text{V}$ (100.0)  | $^{55}\text{Ti}$ (100.0) |
| $^{56}\text{Mn}$             | $^{56}\text{Cr}$ (100.0)                         | $^{56}\text{V}$ (100.0)  | $^{56}\text{Ti}$ (100.0) |
| $^{57}\text{Fe}$             | $^{57}\text{Mn}$ (100.0)                         | $^{57}\text{Cr}$ (100.0) | $^{57}\text{V}$ (100.0)  |
| $^{58}\text{Fe}$             | $^{58}\text{Mn}$ (100.0)                         | $^{58}\text{Cr}$ (100.0) | $^{58}\text{V}$ (100.0)  |
| $^{59}\text{Fe}$             | $^{59}\text{Mn}$ (100.0)                         | $^{59}\text{Cr}$ (100.0) | $^{59}\text{V}$ (100.0)  |
| $^{60}\text{Fe}$             | $^{60}\text{Mn}$ (100.0)                         | $^{60}\text{Cr}$ (100.0) | $^{60}\text{V}$ (100.0)  |
