# Supplementary material for: Cosmic-ray propagation with DRAGON2: II. Nuclear interactions with the interstellar gas
Source: arXiv:1711.09616 ancillary file (2018-07-10)
Supplement: Supplementary file 2 [file isotope-list.pdf]

## A List of isotopes propagated in DRAGON2

| Nucleus          | Intermediate lived nuclei with the branching ratio in %                                                                                                                                                                                                                                                                     |
|------------------|-----------------------------------------------------------------------------------------------------------------------------------------------------------------------------------------------------------------------------------------------------------------------------------------------------------------------------|
| <sup>4</sup> He  | <sup>8</sup> Li <sup>8</sup> B <sup>9</sup> C(100) <sup>8</sup> He(84) <sup>9</sup> Li(50.8) <sup>12</sup> N(3.5) <sup>11</sup> Li(1.9) <sup>12</sup> B(1.6)<br><sup>12</sup> Be(1.59) <sup>14</sup> Be(0.08)                                                                                                               |
| <sup>6</sup> Li  | <sup>6</sup> He(100) <sup>11</sup> Li(1)                                                                                                                                                                                                                                                                                    |
| <sup>7</sup> Li  | <sup>8</sup> He(16) <sup>11</sup> Be(2.95) <sup>11</sup> Li(0.234)                                                                                                                                                                                                                                                          |
| <sup>9</sup> Be  | <sup>9</sup> Li(49.2) <sup>11</sup> Li(4.1)                                                                                                                                                                                                                                                                                 |
| <sup>10</sup> B  | <sup>10</sup> C(100)                                                                                                                                                                                                                                                                                                        |
| <sup>11</sup> B  | <sup>11</sup> C(100) <sup>11</sup> Be(9.71) <sup>11</sup> Li(7.84) <sup>12</sup> Be(0.52)                                                                                                                                                                                                                                   |
| <sup>12</sup> C  | <sup>12</sup> B(98.4) <sup>12</sup> Be(97.89) <sup>12</sup> N(96.5) <sup>13</sup> O(10.9) <sup>14</sup> Be(5.15) <sup>13</sup> B(0.28)                                                                                                                                                                                      |
| <sup>13</sup> C  | <sup>13</sup> N(100) <sup>13</sup> B(99.72) <sup>13</sup> O(89.1) <sup>14</sup> Be(81.62) <sup>14</sup> B(6.04) <sup>17</sup> Ne(2.7) <sup>15</sup> B(0.4)<br><sup>17</sup> B(0.4)                                                                                                                                          |
| <sup>14</sup> N  | <sup>14</sup> O(100)                                                                                                                                                                                                                                                                                                        |
| <sup>15</sup> N  | <sup>15</sup> C <sup>15</sup> O(100) <sup>16</sup> C(97.9) <sup>17</sup> B(72.68) <sup>15</sup> B(6)                                                                                                                                                                                                                        |
| <sup>16</sup> O  | <sup>16</sup> N(100) <sup>17</sup> Ne(96) <sup>17</sup> N(95) <sup>18</sup> C(29.925) <sup>17</sup> C(29.08) <sup>20</sup> Na(25) <sup>20</sup> Mg(24.25)<br><sup>17</sup> B(22.76) <sup>19</sup> C(6.65) <sup>16</sup> C(2.1)                                                                                              |
| <sup>17</sup> O  | <sup>17</sup> F(100) <sup>18</sup> N(10.9) <sup>18</sup> C(9.04) <sup>19</sup> C(5.47) <sup>17</sup> N(5) <sup>17</sup> C(3.58) <sup>17</sup> Ne(1.3)<br><sup>17</sup> B(0.79) <sup>21</sup> Mg(0.5) <sup>22</sup> Si(0.16)                                                                                                 |
| <sup>18</sup> O  | <sup>18</sup> F <sup>18</sup> Ne <sup>19</sup> Na(100) <sup>18</sup> N(76.9) <sup>19</sup> B(61.26) <sup>19</sup> N(54.6) <sup>18</sup> C(52.68) <sup>20</sup> C(39.31)                                                                                                                                                     |
| <sup>19</sup> F  | <sup>19</sup> O <sup>19</sup> Ne(100) <sup>20</sup> N(57) <sup>20</sup> C(48.65) <sup>19</sup> N(45.4) <sup>19</sup> C(20.88) <sup>20</sup> Mg(3)                                                                                                                                                                           |
| <sup>20</sup> Ne | <sup>20</sup> O <sup>20</sup> F(100) <sup>21</sup> N(80) <sup>20</sup> Na(75) <sup>20</sup> Mg(72.75) <sup>20</sup> N(43) <sup>21</sup> Mg(32.6)<br><sup>22</sup> Si(12.13) <sup>20</sup> C(12.04) <sup>22</sup> Al(2.5)                                                                                                    |
| <sup>21</sup> Ne | <sup>21</sup> F <sup>21</sup> O <sup>21</sup> Na(100) <sup>21</sup> Mg(66.9) <sup>22</sup> N(54.88) <sup>22</sup> O(30.88) <sup>22</sup> Si(21.95)<br><sup>21</sup> N(20) <sup>22</sup> F(11) <sup>23</sup> O(3.41) <sup>22</sup> Al(0.8)                                                                                   |
| <sup>22</sup> Ne | <sup>22</sup> Mg(100) <sup>22</sup> Al(96.7) <sup>22</sup> F(89) <sup>22</sup> O(69.42) <sup>22</sup> Si(65.76) <sup>22</sup> N(45.12)<br><sup>23</sup> O(37.25) <sup>23</sup> F(14) <sup>24</sup> O(8) <sup>23</sup> Al(8)                                                                                                 |
| <sup>23</sup> Na | <sup>23</sup> Ne <sup>23</sup> Mg(100) <sup>23</sup> Al(92) <sup>23</sup> F(86) <sup>23</sup> O(59.34) <sup>24</sup> O(52.36) <sup>24</sup> Si(8)<br><sup>24</sup> F(5.9)                                                                                                                                                   |
| <sup>24</sup> Mg | <sup>24</sup> Ne <sup>24</sup> Al(99.96) <sup>24</sup> F(94.1) <sup>24</sup> Si(91.97) <sup>24</sup> O(39.52) <sup>25</sup> Si(36.81)<br><sup>25</sup> F(24) <sup>26</sup> F(1)                                                                                                                                             |
| <sup>25</sup> Mg | <sup>25</sup> Ne <sup>25</sup> Na <sup>25</sup> Al(100) <sup>25</sup> F(76) <sup>25</sup> Si(63.19) <sup>26</sup> F(32.09) <sup>27</sup> S(2)<br><sup>26</sup> P(0.9) <sup>26</sup> Ne(0.13)                                                                                                                                |
| <sup>26</sup> Mg | <sup>26</sup> Na(100) <sup>26</sup> Ne(99.87) <sup>26</sup> F(67.91) <sup>27</sup> Ne(2.13) <sup>27</sup> Si(0.13) <sup>28</sup> Ne(0.03)                                                                                                                                                                                   |
| <sup>27</sup> Al | <sup>27</sup> Mg <sup>27</sup> Si(100) <sup>27</sup> P(99.93) <sup>27</sup> Na(99.87) <sup>27</sup> S(97.93) <sup>27</sup> Ne(97.87)<br><sup>28</sup> Ne(22.42) <sup>28</sup> S(20.7) <sup>28</sup> Na(0.58)                                                                                                                |
| <sup>28</sup> Si | <sup>28</sup> Al <sup>28</sup> P(100) <sup>28</sup> Na(99.42) <sup>28</sup> S(79.3) <sup>28</sup> Ne(77.65)<br><sup>29</sup> S(46.4) <sup>29</sup> Ne(25.9) <sup>29</sup> Na(25.9) <sup>30</sup> Na(1.17) <sup>31</sup> Ar(2.1) <sup>32</sup> Cl(0.054)<br><sup>32</sup> Ar(0.031)                                          |
| <sup>29</sup> Si | <sup>29</sup> Mg <sup>29</sup> Al <sup>29</sup> P(100) <sup>29</sup> Ne(74.1) <sup>29</sup> Na(74.1) <sup>29</sup> S(53.6)<br><sup>30</sup> Na(30) <sup>31</sup> Ar(2.48) <sup>31</sup> Na(0.9)                                                                                                                             |
| <sup>30</sup> Si | <sup>30</sup> Al <sup>30</sup> P <sup>30</sup> S(100) <sup>30</sup> Mg(99.94) <sup>30</sup> Na(68.79) <sup>31</sup> Ar(55.29)<br><sup>31</sup> Na(39) <sup>32</sup> Na(10.41) <sup>31</sup> Mg(3.27) <sup>31</sup> Al(1.6) <sup>31</sup> Cl(0.7) <sup>33</sup> Na(0.393)<br><sup>32</sup> Mg(0.038) <sup>34</sup> Na(0.019) |

| Nucleus          | Intermediate lived nuclei with the branching ratio in %                                                                                                                                                                                                                                                                                      |
|------------------|----------------------------------------------------------------------------------------------------------------------------------------------------------------------------------------------------------------------------------------------------------------------------------------------------------------------------------------------|
| <sup>31</sup> P  | <sup>31</sup> S(100) <sup>31</sup> Cl(99.3) <sup>31</sup> Al(98.4) <sup>31</sup> Mg(93.73) <sup>31</sup> Na(60.02)<br><sup>32</sup> Ar(43.01) <sup>31</sup> Ar(40.14) <sup>32</sup> Na(25.28) <sup>33</sup> Na(13.23) <sup>32</sup> Mg(3.04) <sup>34</sup> Na(1.54)<br><sup>32</sup> Al(0.7) <sup>32</sup> Cl(0.026) <sup>33</sup> Mg(0.012) |
| <sup>32</sup> S  | <sup>32</sup> Cl(99.92) <sup>32</sup> Al(99.3) <sup>32</sup> Mg(96.92) <sup>32</sup> Na(65.81)<br><sup>32</sup> Ar(56.95) <sup>34</sup> Na(52.04) <sup>33</sup> Na(50) <sup>33</sup> Ar(38.7) <sup>33</sup> Mg(23.88)                                                                                                                        |
| <sup>33</sup> S  | <sup>33</sup> Si <sup>33</sup> Cl(100) <sup>33</sup> Al(91.5) <sup>33</sup> Mg(75.94) <sup>33</sup> Ar(61.3)<br><sup>33</sup> Na(27.34) <sup>34</sup> Na(15.77) <sup>34</sup> Mg(12.5) <sup>34</sup> Al(12.5) <sup>35</sup> Na(6.5) <sup>35</sup> Mg(6.5)                                                                                    |
| <sup>34</sup> S  | <sup>34</sup> Si(100) <sup>34</sup> P(100) <sup>34</sup> Ar(100) <sup>34</sup> Cl(99.92) <sup>34</sup> Mg(87.5) <sup>34</sup> Al(87.5)<br><sup>35</sup> Na(59.85) <sup>35</sup> Mg(59.85) <sup>36</sup> Al(31) <sup>34</sup> Na(30.62) <sup>35</sup> Al(29.89) <sup>35</sup> Si(5.26)<br><sup>35</sup> K(0.37) <sup>35</sup> Ca(0.37)        |
| <sup>36</sup> S  | <sup>36</sup> P(100) <sup>36</sup> Si(88) <sup>36</sup> Al(60.72) <sup>37</sup> Si(17)                                                                                                                                                                                                                                                       |
| <sup>35</sup> Cl | <sup>35</sup> P <sup>35</sup> Ar(100) <sup>35</sup> K(99.63) <sup>35</sup> Ca(99.63) <sup>35</sup> Si(94.74)<br><sup>35</sup> Al(70.11) <sup>36</sup> Ca(56.82) <sup>35</sup> Na(33.65) <sup>35</sup> Mg(33.65) <sup>36</sup> Al(37.21) <sup>36</sup> Si(11.37)                                                                              |
| <sup>37</sup> Cl | <sup>37</sup> P <sup>37</sup> S(100) <sup>37</sup> Si(83) <sup>38</sup> P(12)                                                                                                                                                                                                                                                                |
| <sup>36</sup> Ar | <sup>36</sup> K(99.95) <sup>37</sup> Ca(74.7) <sup>36</sup> Ca(43.18) <sup>40</sup> Sc(0.017) <sup>40</sup> Ti(0.01)                                                                                                                                                                                                                         |
| <sup>38</sup> Ar | <sup>38</sup> S <sup>38</sup> Cl <sup>38</sup> K <sup>38</sup> Ca <sup>39</sup> Sc <sup>39</sup> Ti (100) <sup>38</sup> P (88) <sup>39</sup> P(26)                                                                                                                                                                                           |
| <sup>40</sup> Ar | <sup>40</sup> S <sup>40</sup> Cl (100) <sup>40</sup> P(70) <sup>41</sup> P(30)                                                                                                                                                                                                                                                               |
| <sup>39</sup> K  | <sup>39</sup> S <sup>39</sup> Cl <sup>39</sup> Ca (100) <sup>39</sup> P (74) <sup>40</sup> P (30) <sup>40</sup> Sc (0.44) <sup>40</sup> Ti(0.25)                                                                                                                                                                                             |
| <sup>41</sup> K  | <sup>41</sup> S <sup>41</sup> Cl (100) <sup>41</sup> P(70) <sup>42</sup> P(52)                                                                                                                                                                                                                                                               |
| <sup>40</sup> Ca | <sup>41</sup> Ti (100) <sup>40</sup> Sc (99.54) <sup>40</sup> Ti(56.74)                                                                                                                                                                                                                                                                      |
| <sup>42</sup> Ca | <sup>42</sup> Cl <sup>42</sup> Sc <sup>42</sup> Ti(100) <sup>42</sup> S(96) <sup>43</sup> P (96) <sup>42</sup> P (48) <sup>43</sup> Ti (40) <sup>43</sup> Cr (23)                                                                                                                                                                            |
| <sup>43</sup> Ca | <sup>43</sup> Cl <sup>43</sup> Ar <sup>43</sup> Ti(100) <sup>43</sup> S (60) <sup>44</sup> S (24.56) <sup>44</sup> Cl (8) <sup>44</sup> Cr (7) <sup>45</sup> S (4.32)                                                                                                                                                                        |
| <sup>44</sup> Ca | <sup>44</sup> Ar <sup>44</sup> K(100) <sup>44</sup> Cl(92) <sup>44</sup> S(75.44) <sup>45</sup> S (60.72) <sup>45</sup> Cl (24)                                                                                                                                                                                                              |
| <sup>46</sup> Ca | <sup>46</sup> Ar <sup>46</sup> K (100) <sup>46</sup> Cl(40) <sup>47</sup> Cl(3.97) <sup>47</sup> Ar(1)                                                                                                                                                                                                                                       |
| <sup>48</sup> Ca | <sup>48</sup> K (98.86) <sup>49</sup> Sc(86)                                                                                                                                                                                                                                                                                                 |
| <sup>45</sup> Sc | <sup>45</sup> Ar <sup>45</sup> K <sup>45</sup> Ti <sup>45</sup> V(100) <sup>45</sup> Cl(76) <sup>45</sup> Cr(73) <sup>46</sup> Cl(60) <sup>45</sup> S(34.96)<br><sup>46</sup> Mn(22) <sup>46</sup> Fe(22)                                                                                                                                    |
| <sup>46</sup> Ti | <sup>46</sup> V <sup>46</sup> Cr(100) <sup>46</sup> Mn(78) <sup>47</sup> Mn(3.4)                                                                                                                                                                                                                                                             |
| <sup>47</sup> Ti | <sup>47</sup> K <sup>47</sup> V <sup>47</sup> Cr(100) <sup>47</sup> Ar(99) <sup>47</sup> Mn <sup>47</sup> Fe(96.6) <sup>47</sup> Cl(16)<br><sup>48</sup> Fe(3.75) <sup>48</sup> K(1.14) <sup>48</sup> Mn(0.3)                                                                                                                                |
| <sup>49</sup> Ti | <sup>49</sup> Ca <sup>49</sup> Ti(100) <sup>50</sup> K(29) <sup>49</sup> K(14)                                                                                                                                                                                                                                                               |
| <sup>50</sup> Ti | <sup>50</sup> Ca <sup>50</sup> Sc(100) <sup>50</sup> K(71) <sup>51</sup> K(47) <sup>52</sup> K(21)                                                                                                                                                                                                                                           |
| <sup>51</sup> V  | <sup>51</sup> Ca <sup>51</sup> Sc <sup>51</sup> Ti(100) <sup>52</sup> K(64.3) <sup>51</sup> K(53) <sup>53</sup> K(18.34) <sup>52</sup> Ca(2)                                                                                                                                                                                                 |
| <sup>50</sup> Cr | <sup>50</sup> Mn <sup>50</sup> Fe(100) <sup>50</sup> Co(46)                                                                                                                                                                                                                                                                                  |
| <sup>52</sup> Cr | <sup>52</sup> Sc <sup>52</sup> Ti <sup>52</sup> V <sup>52</sup> Co(100) <sup>52</sup> Ca(98) <sup>52</sup> Ni(83) <sup>53</sup> K(70.46)<br><sup>53</sup> Ni(45) <sup>53</sup> Ca(30) <sup>52</sup> K(14.7)                                                                                                                                  |
| <sup>53</sup> Cr | <sup>53</sup> Sc <sup>53</sup> Ti <sup>53</sup> V(100) <sup>53</sup> Ca(70) <sup>53</sup> K(11.2)                                                                                                                                                                                                                                            |
| <sup>54</sup> Cr | <sup>54</sup> Sc <sup>54</sup> Ti <sup>54</sup> V(100)                                                                                                                                                                                                                                                                                       |
| <sup>55</sup> Mn | <sup>55</sup> Sc <sup>55</sup> Ti <sup>55</sup> V <sup>55</sup> Cr(100)                                                                                                                                                                                                                                                                      |
| <sup>54</sup> Fe | <sup>54</sup> Co <sup>54</sup> Ni(100)                                                                                                                                                                                                                                                                                                       |
| <sup>56</sup> Fe | <sup>56</sup> Ti <sup>56</sup> V <sup>56</sup> Cr <sup>56</sup> Co(100)                                                                                                                                                                                                                                                                      |
| <sup>57</sup> Fe | <sup>57</sup> Ti <sup>57</sup> V <sup>57</sup> Cr <sup>57</sup> Mn <sup>57</sup> Co(100)                                                                                                                                                                                                                                                     |
| <sup>58</sup> Fe | <sup>58</sup> V <sup>58</sup> Cr <sup>58</sup> Mn <sup>58</sup> Co(100)                                                                                                                                                                                                                                                                      |
